# Supplementary material for: Mutation Analysis for Cyber-Physical Systems: Scalable Solutions and Results in the Space Domain
Source: arXiv:2101.05111 source file (2021-08-23)
Supplement: Supplementary file 1 [file appendixFSCIReduced.tex]

\section{Accuracy of uniform FSCI sampling with PrioritizeAndReduce}
\label{appendix:FSCI:reduced}

\begin{table*}[h]
\centering
\scriptsize
\caption{RQ5. CI definition for \APPR Test Suites.}
\label{table:results:ciDefinition} 
\begin{tabular}{|l|l|llllllllll|}
\hline
          &                           & \multicolumn{2}{c}{\GCSP{}} & \multicolumn{2}{c}{\PARAM{}} & \multicolumn{2}{c}{\UTIL{}} & \multicolumn{2}{c}{\MLFS{}{}} & \multicolumn{2}{c|}{\SAIL{}} \\
\hline
Strategy  & Method                    & \#Mutants    & \textbf{$\delta_{acc}$}    & \#Mutants    & \textbf{$\delta_{acc}$}    & \#Mutants    & \textbf{$\delta_{acc}$}   & \#Mutants  & \textbf{$\delta_{acc}$}  & \#Mutants   & \textbf{$\delta_{acc}$}  \\
\hline
$D_J$   & \multirow{4}{*}{CI 0.1}  & 519.1        & 3.55          & 356.7        & 3.62          & 345.8        & 2.54         & 284.6      & 4.07        &    NA         &     NA        \\
$D_O$    &                           				& 518        & 3.55          & 356.7        & 3.62          & 345.8        & 2.54         & 286.1      & 4.07        &       NA     &     NA        \\
$D_E$ &                           					& 449.5        & 3.75          & 356.7        & 3.62          & 345.8        & 2.51         & 259.1      & 4.33        &   1128.8          & 4.78            \\
$D_C$    &                          					 & 448.7        & 3.75          & 356.7        & 3.62          & 343.3        & 2.57         & 258.5      & 4.27        &    1230.8 &   4.88          \\
\hline
$D_J$   & \multirow{4}{*}{CI 0.09} & 667.7        & 3.95          & 439.5        & 3.78          & 424.2        & 2.34         & 352.8      & 4.72        &     NA        &    NA         \\
$D_O$    &                          					 & 665.7        & 3.93          & 439.5        & 3.78          & 424.2        & 2.34         & 353      & 4.72        &        NA     &       NA      \\
$D_E$ &                           					& 567.2        & 3.14          & 439.5        & 3.78          & 422.3         & 2.14         & 316.5      & 5.19        &  1652.2           & 4.88            \\
$D_C$    &                          					 & 566.3        & 3.14          & 439.5        & 3.78          & 421.3        & 2.12         & 316.6      & 5.19        &   1832.8          &  4.92           \\
\hline
$D_J$   & \multirow{4}{*}{CI 0.08} &885.8        & 1.94          & 558.2        & 3.40          & 535.4        & 2.30         & 450.7        & 3.66        &      NA       &       NA      \\
$D_O$    &                           					& 883.8        & 2.04          & 558.2        & 3.40          & 535.4        & 2.30     & 451      & 3.66        &      NA       &   NA          \\
$D_E$ &                          					 & 735.8        & 3.22          & 558.2        & 3.40          & 531.2        & 2.79         & 392.7      & 4.40        &      NA       &   4.24          \\
$D_C$    &                          					 & 734        & 3.23          & 558.2        & 3.40          & 529.9        & 2.76         & 393.4      & 3.85        &     NA        &     4.30        \\
\hline
$D_J$   & \multirow{4}{*}{CI 0.07} & 1235.4       & 2.42          & 730.3        & 2.33          & 709.5        & 2.76         & 599.9      & 2.61       &      NA       &      NA       \\
$D_O$    &                           					& 1231.5       & 2.53          & 730.3        & 2.33          & 709.5        & 2.76         & 600.8        & 2.61        &      NA       &    NA         \\
$D_E$ &                           					& 993.1       & 1.88          & 730.3        & 2.33          & 704.7        & 2.81         & 511        & 4.11        &       NA      &    NA        \\
$D_C$    &                           					& 990.4       & 1.91          & 730.3        & 2.33          & 702          & 2.81         & 508.7      & 4.12        &    NA         &    NA        \\
\hline
$D_J$   & \multirow{4}{*}{CI 0.06} & 1860.4       & 1.92          & 996.8        & 2.26          & 963          & 2.84         & 859.2      & 2.20        &    NA         &  NA           \\
$D_O$    &                          					 & 1852.5       & 1.98          & 996.8        & 2.26          & 963        & 2.84         & 860      & 2.20        &       NA      &      NA       \\
$D_E$ &                           					& 1416       & 1.68          & 996.8        & 2.26          & 955.8        & 2.85         & 709.7      & 2.39        &      NA       &       NA      \\
$D_C$    &                        					   & 1410.9       & 1.74          & 996.8        & 2.26          & 951.9        & 2.85         & 707.8      & 2.39        &     NA        &   NA          \\
\hline
$D_J$   & \multirow{4}{*}{CI 0.05} & NA           & 1.69          & 1438         & 1.61          & 1392       & 2.58         & 1273.4     & 2.24        &    NA         &       NA      \\
$D_O$    &                         					  & NA           & 1.63          & 1438         & 1.61          & 1392       & 2.58         & 1275.7     & 2.20        &     NA        &      NA       \\
$D_E$ &                          					 & 2197       & 1.22          & 1438         & 1.61          & 1377.3       & 2.54         & 1038.6     & 2.18        &       NA      &       NA      \\
$D_C$    &                        					   & 2187.9       & 1.23          & 1438         & 1.61          & 1370         & 2.48         & 1035.8     & 2.10        &   NA          &     NA       \\
\hline
\end{tabular}
\end{table*}
